# Supplementary material for: Identifying and Mitigating Position Bias of Multi-image Vision-Language Models
Source: arXiv:2503.13792 source file (2025-03-18)
Supplement: Supplementary file 1 [file X_suppl.tex]

\clearpage
\setcounter{page}{1}
\maketitlesupplementary

\section*{A. Experimental Details}
Here, we provide a detailed description of the models, benchmarks, and evaluation details employed for this work.

\noindent\textbf{Models}. We provide an overview of each LVLM along with our specifications.

\noindent 1) \textbf{OpenFlamingo}~\citep{awadalla2023openflamingo} represents a pioneering effort in the realm of multi-image LVLMs, serving as the open-source reproduction of Flamingo~\citep{alayrac2022flamingo}. It maintains an almost identical architecture and training framework to the original. For our evaluation, we utilize the second version, OFv2, and conduct experiments on a model with 9 billion parameters.

\noindent 2) \textbf{Idefics2}~\citep{laurenccon2024matters} is an 8-billion-parameter multi-image model pre-trained on newly collected interleaved web documents~\citep{laurenccon2024obelics} and instruction datasets~\citep{laurenccon2024matters} from Huggingface. For our experiments, we adhere to its default settings, with the exception of disabling sub-image splitting for fairness.

\noindent 3) \textbf{LLaVA-NeXT-Interleave}~\citep{li2024llava} is a recently developed model designed to enhance the multi-image, multi-frame, and multi-view reasoning capabilities of the LLaVA family. In this study, we utilize its 7-billion-parameter variant.

\noindent 4) \textbf{InternVL2}~\citep{chen2024internvl} is a flexible multi-modal model that utilizes progressive alignment with large language models, ranging from 1 billion to 108 billion parameters. Here, we use its 8-billion-parameter variant, which employs dynamic resolution.

\noindent 5) \textbf{VILA}~\citep{lin2024vila} is a meticulously designed model that employs an empirically optimized pre-training strategy by reblending interleaved and image-text pair data. In this study, we utilize its 13-billion-parameter variant with 8-bit quantization.

\noindent 6) \textbf{Mantis}~\citep{jiang2024mantis} is an 8-billion-parameter state-of-the-art family enhanced from existing models through multi-image instruction tuning. Here, we select Mantis-Idefics2, which is directly fine-tuned from Idefics2~\citep{laurenccon2024matters}. 

\noindent \textbf{Benchmarks}. We introduce the selected benchmarks here. In \hyperref[subsec:motivation]{§3.1} and \hyperref[subsec:robustness]{§5.1}, to explore the impact of changing positions on predictions, we define position-agnostic tasks, which refer to tasks where changing the position does not alter the semantics of the question. Here, we list the position-agnostic tasks for each benchmark.

\noindent 1) \textbf{BLINK}~\citep{fu2024blink} is a novel benchmark comprising 14 tasks that can be effortlessly solved by humans yet present challenges for LVLMs. 

\noindent 2) \textbf{MuirBench}~\citep{wang2024muirbench} is a comprehensive benchmark consisting of 12 tasks designed to evaluate the multi-image understanding capabilities of existing LVLMs. 

\noindent 3) \textbf{MIRB}~\citep{zhao2024benchmarking} is a multi-image benchmark developed to assess the relational reasoning capabilities of LVLMs. 

\noindent 4) \textbf{Mantis-Eval}~\citep{jiang2024mantis} is a compact test set designed for the Mantis family. Additionally, for comprehensiveness, we include some samples from Mantis-Instruct and ensure that they do not overlap with other benchmarks.

\noindent \textbf{Evaluation}. We uniformly employ LLM-as-a-judge for evaluation throughout the study. Specifically, we utilize GPT-4, providing it with the question, ground truth, and model prediction for each example, and instructing it to assess the correctness of the response. To maintain evaluation consistency, we use the default system prompt and set the temperature to 0, thereby employing greedy search decoding.
\section*{B. Limitations and Failure Cases}
\noindent\textbf{High sensitivety to hyperparameters}. 
The proposed SoFA effectively mitigates position bias, yet its performance is highly sensitive to the choice of $\sigma$, which necessitates a small labeled validation set for calibration (32-shot in this study). Through our ablation study, we empirically demonstrate that no single global optimal $\sigma$ is suitable across all tasks; instead, the optimal choice of $\sigma$ is task-dependent and varies according to the specific characteristics of the task at hand. In future work, we could explore learning $\sigma$ through gradient-based methods or directly fine tune the attention mask. Additionally, designing separate $\sigma$ for each layer may be considered for better performance.

\noindent\textbf{Limited to autoregressive models}. SoFA is applicable to the vast majority of LVLMs that employ an autoregressive framework, wherein visual tokens are concatenated with text tokens and processed through the input layer. However, SoFA may not be suitable for certain specialized or custom architectures. For example, Flamingo~\citep{alayrac2022flamingo} adopts a different approach by using image-text cross-attention, where text functions as the query and the image as both the key and value for interaction. Given the distinct nature of this architecture, we have not addressed it in this work and consider it as part of future research.
\section*{C. Societal Broader Impact}
Our work has positive broader impacts. Intuitively, the position bias in LVLMs could be considered an imitation of human psychology, where people tend to selectively remember certain images while forgetting others while faced with multiple ones, a phenomenon called serial-position effect~\citep{ebbinghaus1913contribution, murdock1962serial}. We argue that this imbalanced reasoning capability across positions leads LVLMs to 1) potentially miss key information, impairing their performance and 2) produce unreliable responses influenced by image order. This is detrimental to various multi-image applications such as scene understanding and visual analogy. Our proposed SoFA, by slightly modifying attention, effectively mitigates this issue. Despite being an inference-only method, we hope our approach can also inspire the community to devise more remedies during the training stage.

Currently, we have not identified any significant negative impacts. However, this needs to be reassessed in the future due to objective factors such as the availability of datasets and models.
